# Supplementary material for: Co-clustering of Spatially Resolved Transcriptomic Data
Source: arXiv:2110.04872 source file (2022-09-14)
Supplement: Supplementary file 1 [file Sottosanti_Risso_Supplementary_arXiv_9-10-2021.pdf]

# Co-clustering of Spatially Resolved Transcriptomic Data Supplementary Material

A. Sottosanti<sup>1</sup> and D. Risso<sup>1</sup>

<sup>1</sup>University of Padova, Department of Statistical Sciences,  
via Cesare Battisti 241-243, Padova, Italy

October 27, 2021

Address for correspondence: `andrea.sottosanti@unipd.it`

## 1 Derivation of the ICL for SpaRTaCo

Let  $m$  be the current model, and  $K$  and  $R$  be the number of row and column clusters. The *integrated classification likelihood* (Biernacki *and others*, 2000) is defined as

$$\begin{aligned} p(\mathbf{X}, \mathbf{Z}, \mathbf{W}; m, K, R) &= p(\mathbf{X}|\mathbf{Z}, \mathbf{W}; m, K, R)p(\mathbf{Z}, \mathbf{W}; m, K, R) \\ &= p(\mathbf{X}|\mathbf{Z}, \mathbf{W}; m, K, R)p(\mathbf{Z}; m, K)p(\mathbf{W}; m, R). \end{aligned} \quad (1)$$

According to Biernacki *and others* (2000), the conditional distribution of  $\mathbf{X}$  given the clustering labels can be approximated as

$$\log p(\mathbf{X}|\mathbf{Z}, \mathbf{W}; m, K, R) \approx \max_{\Theta} \log p(\mathbf{X}|\mathbf{Z}, \mathbf{W}; \Theta, m, K, R) + \frac{\lambda_{m,K,R}}{2} \log np,$$

where the first component is the classification log-likelihood evaluated in its maximum, and  $\lambda_{m,K,R}$  is the number of free parameters in model  $m$  with  $K$  and  $R$  clusters. Thus, under the identifiability constraint in Section 3.1,  $\lambda_{m,K,R} = 4KR + \dim(\phi)R$ . The distribution of both  $\mathbf{Z}$  and  $\mathbf{W}$  is Multinomial with probabilities  $1/K$  and  $1/R$ , respectively. It follows that

$$\log p(\mathbf{Z}; m, K) = -n \log K, \quad \log p(\mathbf{W}; m, R) = -p \log R.$$

Finally, taking the logarithm of (1) and replacing  $\mathbf{Z}$  and  $\mathbf{W}$  with their estimates  $\hat{\mathbf{Z}}$  and  $\hat{\mathbf{W}}$ , we obtain the ICL.

## 2 Spatial covariance functions

The following isotropic spatial covariance functions have been employed to generate the spatial experiments proposed in Section 4 of the manuscript:

$$k_1^{\text{true}}(d; \phi_1^{\text{true}} = \{\theta_E\}) = \exp\left(-\frac{d}{\theta_E}\right), \quad k_2^{\text{true}}(d; \phi_2^{\text{true}} = \{\theta_R, \alpha_R\}) = \left(1 + \frac{d^2}{2\alpha_R\theta_R^2}\right)^{-\alpha_R}.$$

$$k_3^{\text{true}}(d; \phi_3^{\text{true}} = \{\theta_G\}) = \exp\left(-\frac{d^2}{2\theta_G^2}\right),$$

$k_1^{\text{true}}(\cdot; \theta_E)$  is the *Exponential* kernel with scale  $\theta_E$ ,  $k_2^{\text{true}}(\cdot; \{\theta_R, \alpha_R\})$  the *Rational Quadratic* kernel with non-negative parameters  $(\alpha_R, \theta_R)$ , and  $k_3^{\text{true}}(\cdot; \theta_G)$  is the *Gaussian* kernel (known also as *Squared Exponential*) with *characteristic length-scale*  $\theta_G$ .

## 3 Covariance matrices of the genes

Here, we describe the main characteristics of the simulated covariance matrices simulated as in Formula (4.7) of the manuscript. The degrees of freedom of a Wishart distribution have to be at least equal to the matrix dimension, that is 200. Both the scales and the degrees of freedom are selected in such a way that the values in  $\Sigma_k^{\text{true}}$  have the same order of magnitude of  $c^{\text{true}}$ . For example, using the illustrated setup, the elements on the diagonals of  $\Sigma_1^{\text{true}}$  and  $\Sigma_2^{\text{true}}$  have expected values 6.3 and 11.5, respectively. The top line of Figure 1 displays the histogram of the diagonal values of a single realization of  $\Sigma_k^{\text{true}}$ , for  $k = 1, 2, 3$ . The values are globally comparable across the three simulations. The bottom line of Figure 1 illustrates the elements out of the diagonal of  $\Sigma_k^{\text{true}}$ . The difference between the first and the two other matrices is graphically visible:  $\Sigma_1^{\text{true}}$  is in fact the one with the smallest covariance values. The second and the third appear similar: in  $\Sigma_2^{\text{true}}$ , the elements out of the diagonal are in the range  $(-3.2, 3.1)$ , while in  $\Sigma_3$  they are in the range  $(-3.88, 3.81)$ .

## 4 Additional figures

This section gives some additional figures from Section 2, 4 and 5 of the manuscript.

### Section 2

Figure 2 gives a representation of the relations across co-clustering models described in Section 2.2 of the manuscript.

### Section 4

Figure 3 shows the results of the model selection performed in Section 4.2 using the ICL criterion. According to the notation defined in Section 4.6 of the manuscript, Figure 4

shows a single realization of  $\mathbf{X}_s$ ,  $\mathbf{X}_b$  and  $\mathbf{X}$  using  $\lambda_s = \lambda_b = \sqrt{0.5}$ . Last, Figure 5 shows the results of the model selection performed in Section 4.7.

## Section 5

Figure 6 displays the genes ordered according to the deviance criterion proposed by Townes *and others* (2019). The red line denotes the number of genes selected for our analysis ( $n = 1000$ ), the blue line is the “ideal” number of genes that should be used ( $n = 200$ ), based on where the deviance curve has a significant change in the decay. Figure 7 and 8 display the conditional distributions of  $\sigma_{kr,i}^2$  given the data and the parameter estimates.

## References

- BIERNACKI, CHRISTOPHE, CELEUX, GILLES AND GOVAERT, GÉRARD. (2000). Assessing a mixture model for clustering with the integrated completed likelihood. *IEEE transactions on pattern analysis and machine intelligence* **22**(7), 719–725.
- TOWNES, F. WILLIAM, HICKS, STEPHANIE C., ARYEE, MARTIN J. AND IRIZARRY, RAFAEL A. (2019). Feature selection and dimension reduction for single-cell rna-seq based on a multinomial model. *Genome biology* **20**(1), 1–16.

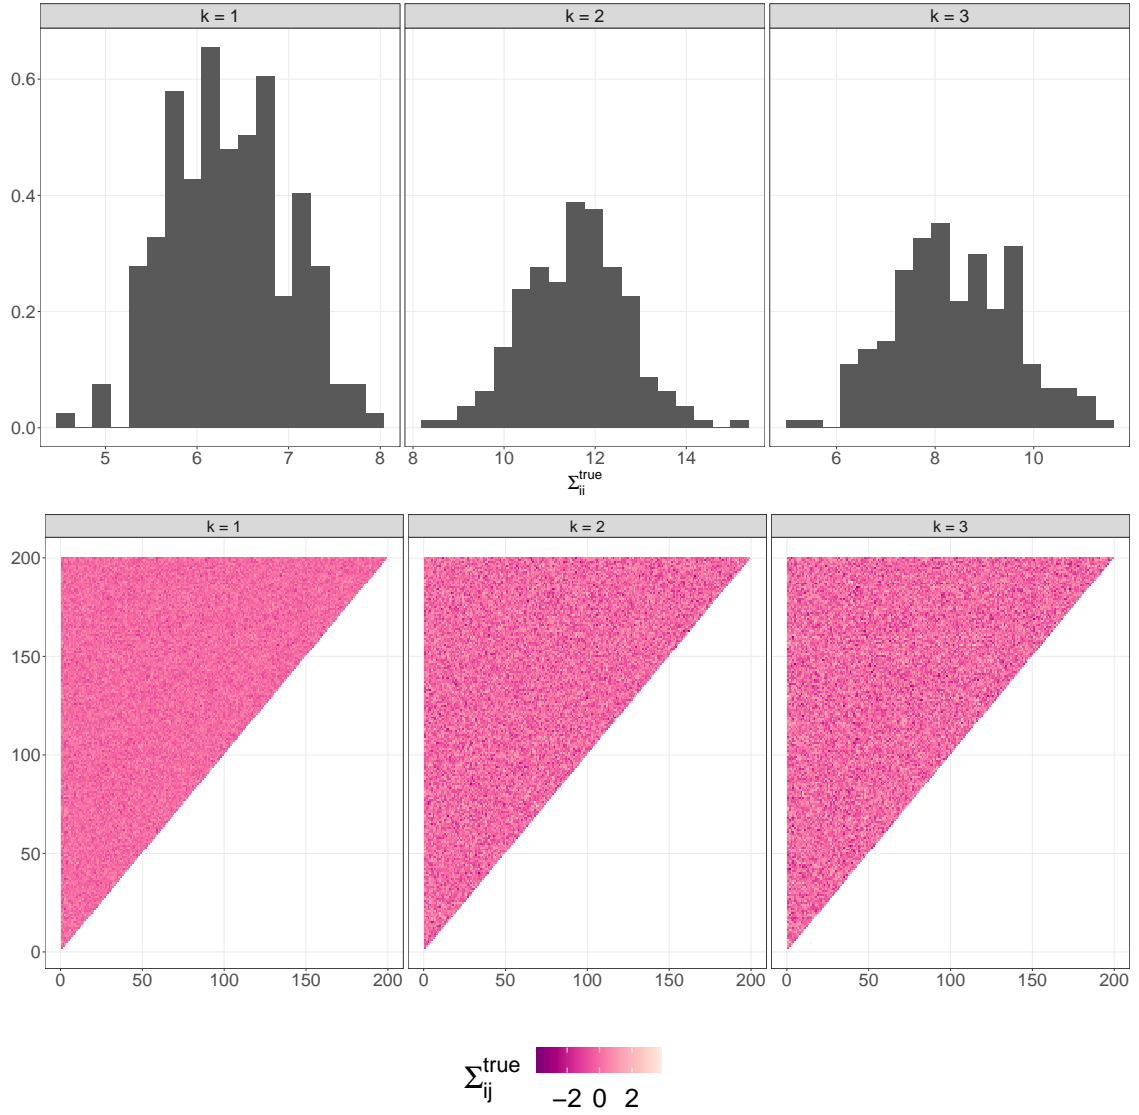

Figure 1: Plot of the row covariance matrices used in Section 2.3 of the manuscript. The top line displays the histogram of the diagonal values of  $\Sigma_k^{\text{true}}$ , the bottom line displays the upper triangular matrix of  $\Sigma_k^{\text{true}}$ , for  $k = 1, 2, 3$ .

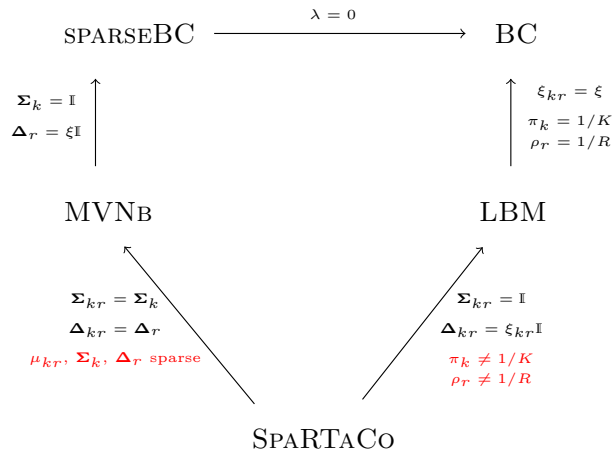

Figure 2: Map of the co-clustering models described in Section 2.2 of the manuscript. An arrow from model A to model B means that B is a special case of A. Details of how to pass from model A to model B are written in black. A red label denotes a difference between two models A and B which does not make B a special case of A.

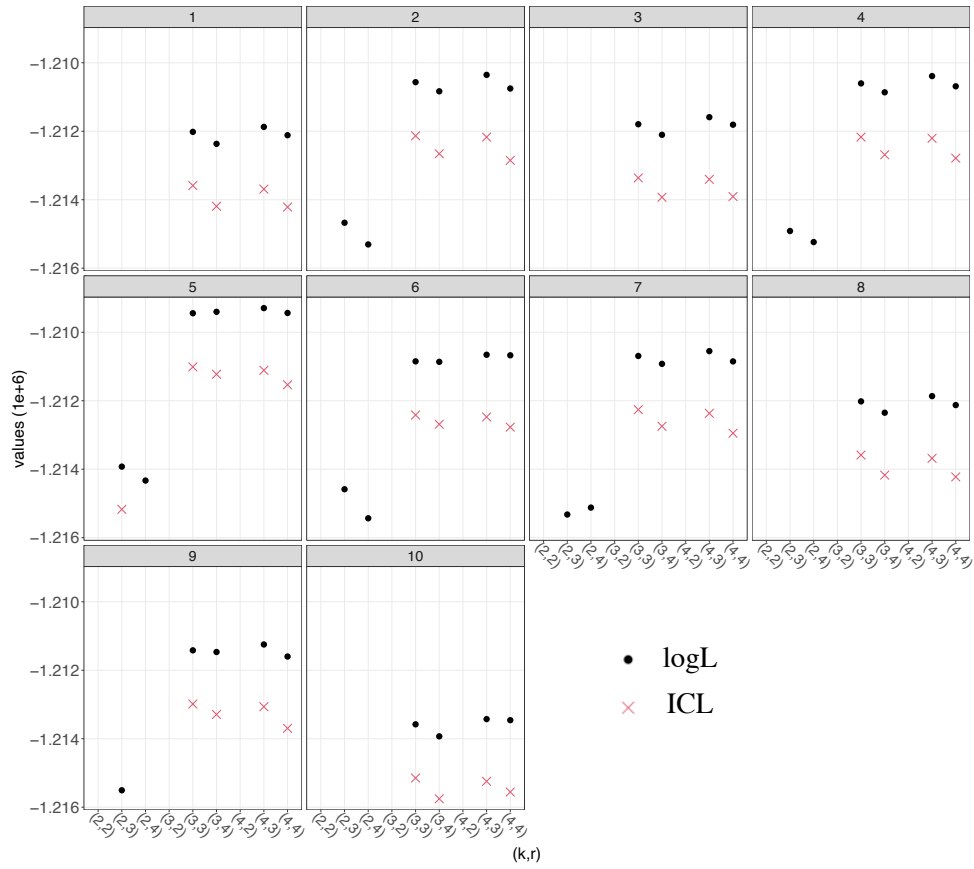

Figure 3: Results of model selection from Scenario 1. The graphs give the log-likelihood and the ICL values obtained from different configurations of SPARTACO on each of the 10 replicates of the experiment. We truncate on purpose the extremes of the y-axis to show only the models with the largest values of log-likelihood and ICL.

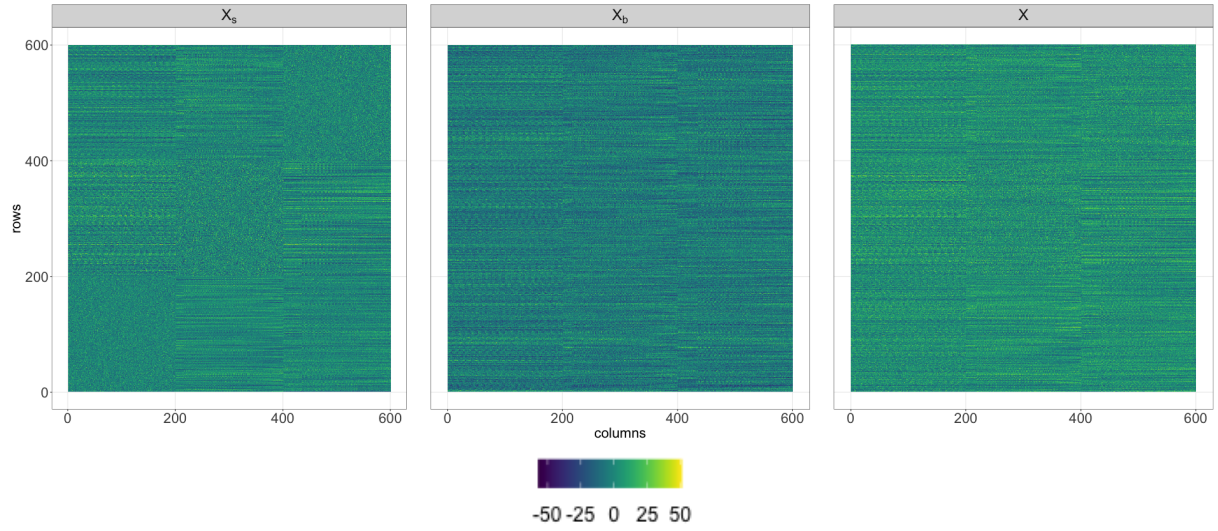

Figure 4: Simulation experiment 4. The matrices  $X_s$ ,  $X_b$  and  $X$  appear from the left to the right, using  $\lambda_s = \lambda_b = \sqrt{0.5}$ .

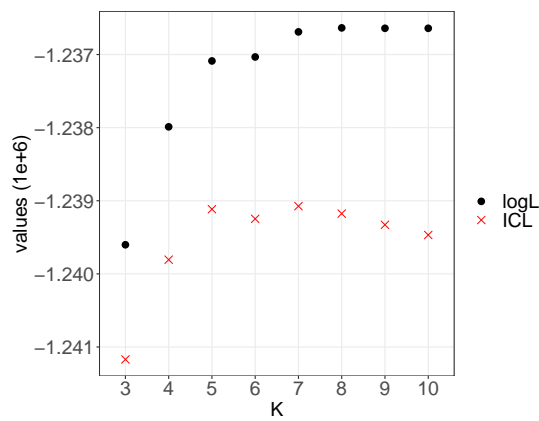

Figure 5: Model selection in Simulation 5. According to the ICL, the best model is the one with  $K = 7$  row clusters. The number of column clusters is fixed to  $R = 3$ .

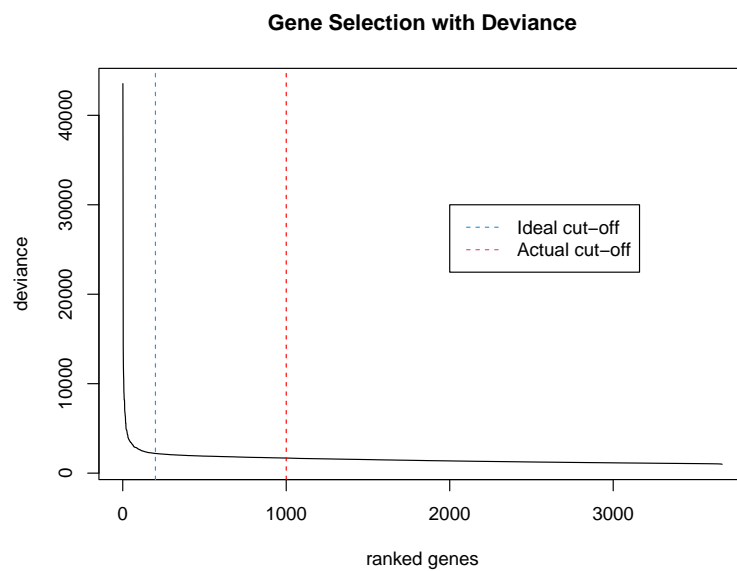

Figure 6: Graph of the genes sorted in decreasing order according to the deviance value. High deviance value are associated to informative genes. Even if from a graphical evaluation the ideal number of genes is around 200, we included in the analysis the 1,000 genes with the largest deviance.



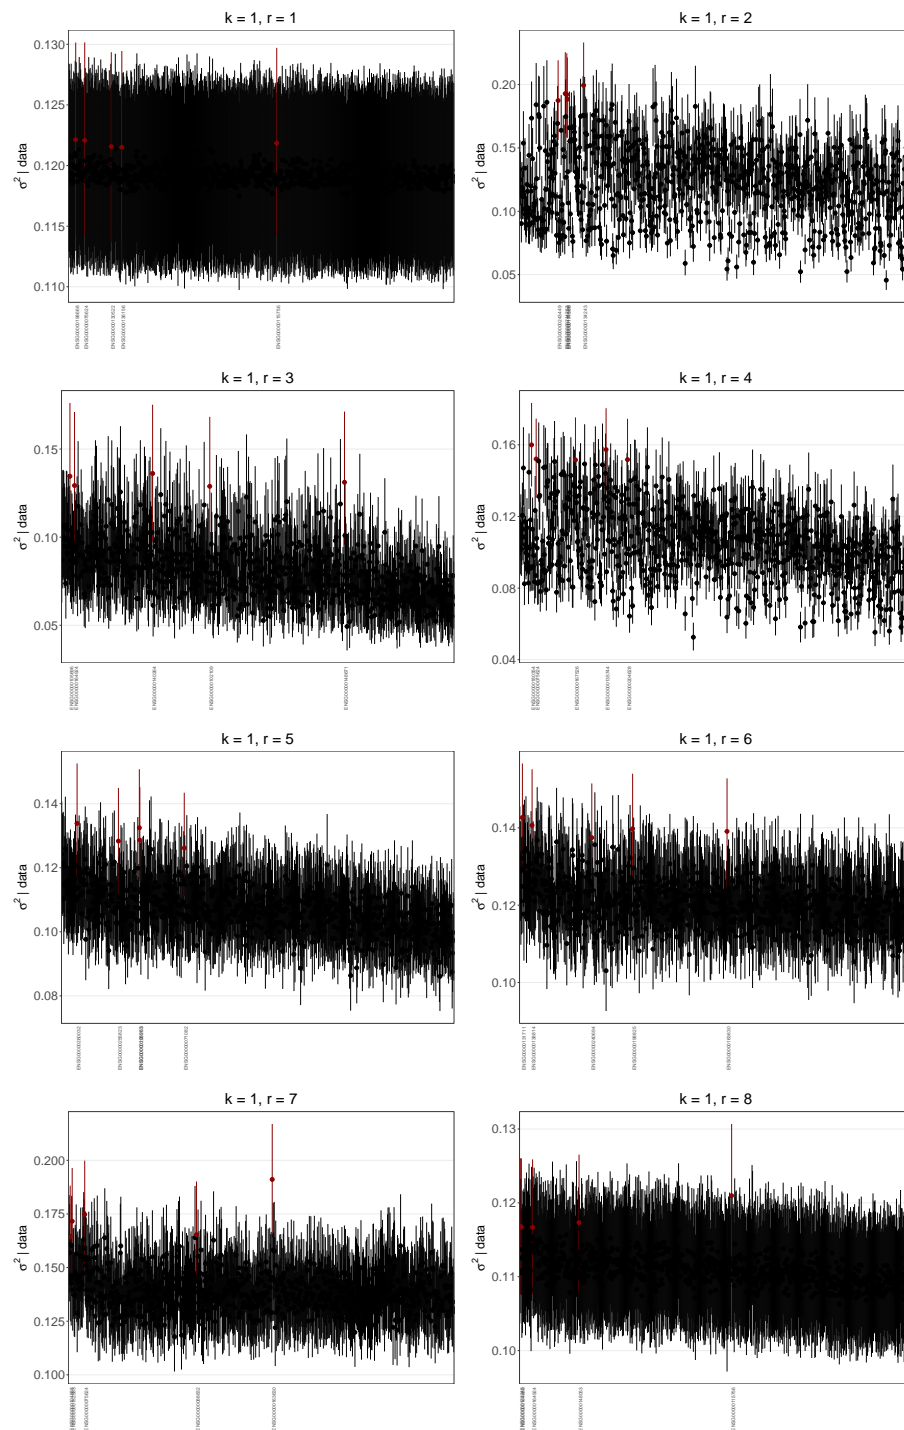

Figure 7: Distribution of  $\sigma^2_{1r,i} | \text{data}$ , where data denotes both the input data and the estimated quantities. The dots denote the expected values and the error bars denote the 95% credible intervals. For each block, the image colours the five genes with the largest expectation in red.

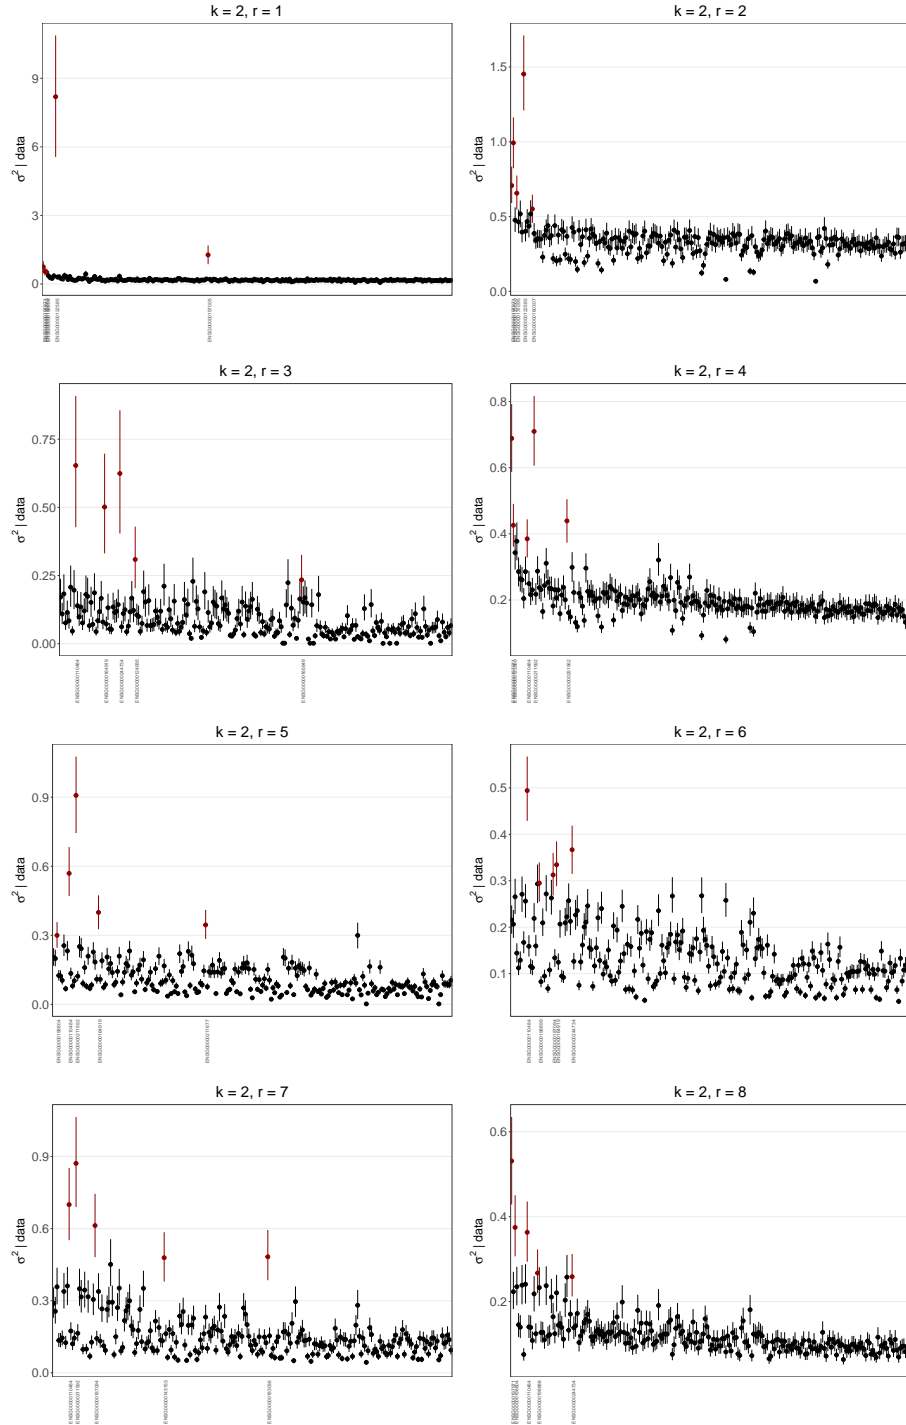

Figure 8: Distribution of  $\sigma^2_{2r,i} | \text{data}$ , where “data” stands for both the input data and the estimated quantities. The dots denote the expected values and the error bars are the 95% credible intervals. For each block, the image colours the five genes with the largest expectation in red.
